# Supplementary material for: LOD-GS: Level-of-Detail-Sensitive 3D Gaussian Splatting for Detail Conserved Anti-Aliasing
Source: arXiv:2507.00554 source file (2025-08-30)
Supplement: Supplementary file 1 [file singlescale_supp.tex]

& \multicolumn{9}{c}{\textbf{PSNR}} \\
 & \scenename{chair}  & \scenename{drums}  & \scenename{ficus}  & \scenename{hotdog}  & \scenename{lego}  & \scenename{materials}  & \scenename{mic}  & \scenename{ship} & \scenename{Average} 
 \\ 
 \hline 
SRN~\cite{srn}&                    29.96  &                    17.18  &                    20.73  &                    26.81  &                    20.85  &                    18.09  &                    26.85  &                    20.60  &  22.26
\\
LLFF~\cite{mildenhall2019local}&                    28.72  &                    21.13  &                    21.79  &                    31.41  &                    24.54  &                    20.72  &                    27.48  &                    23.22  &  24.88
\\
Neural Volumes~\cite{neuralvolumes}&                    28.33  &                    22.58  &                    24.79  &                    30.71  &                    26.08  &                    24.22  &                    27.78  &                    23.93  &   26.05
\\
Plenoxels~\cite{fridovich2022plenoxels} &                             33.98  &                    25.35  &                    31.83  &                    36.43  &                    34.10  &                    29.14  &                    33.26  & 29.62 &  31.71
\\
NeRF~\cite{mildenhall2020nerf} &                    34.17  &                    25.08  &                    30.39  &                    36.82  &                    33.31  &                    30.03  &                    34.78  &                    29.30  &  31.74
\\
DVGO~\cite{sun2022direct} &                    34.09  &                    25.44  &                    32.78  &                    36.74  &                    34.64  &                    29.57  &                    33.20  &                    29.13  &  31.95
\\
MipNeRF~\cite{barron2021mip} &                    \cellcolor{yellow}35.14  &                    25.48  &                    33.29  &                    \cellcolor{orange}37.48  &                    35.70  &                    \cellcolor{orange}30.71  &                    \cellcolor{orange}36.51  &                    \cellcolor{yellow}30.41  & 33.09
\\
TensoRF~\cite{chen2022tensorf} &                    \cellcolor{orange}35.76  &                    \cellcolor{yellow}26.01  &                    \cellcolor{orange}33.99  &                    \cellcolor{yellow}37.41  &                    \cellcolor{red}36.46  &                    \cellcolor{yellow}30.12  &                    34.61  &                    \cellcolor{orange}30.77  & \cellcolor{yellow}33.14
\\
Instant-ngp~\cite{muller2022instant} &                    35.00  &                    \cellcolor{orange}26.02  &                    \cellcolor{yellow}33.51  &                    37.40  &                    \cellcolor{orange}36.39  &                    29.78  &                    \cellcolor{yellow}36.22  &                    \cellcolor{red}31.10  & \cellcolor{orange}33.18
\\
\hline
Tri-MipRF (Ours) &                    \cellcolor{red}36.10  &                    \cellcolor{red}26.59  &                    \cellcolor{red}34.51  &                    \cellcolor{red}38.54  &                    \cellcolor{yellow}36.15  &                    \cellcolor{red}30.73  &                    \cellcolor{red}37.75  &                    28.78 & \cellcolor{red}33.65  
\\

\multicolumn{9}{c}{} \\
 & \multicolumn{9}{c}{\textbf{SSIM}} \\
 & \scenename{chair}  & \scenename{drums}  & \scenename{ficus}  & \scenename{hotdog}  & \scenename{lego}  & \scenename{materials}  & \scenename{mic}  & \scenename{ship} & \scenename{Average} 

\\ 
\hline 
SRN~\cite{srn}&                    0.910  &                    0.766  &                    0.849  &                    0.923  &                    0.809  &                    0.808  &                    0.947  &                    0.757  & 0.846
\\
LLFF~\cite{mildenhall2019local}&                    0.948  &                    0.890  &                    0.896  &                    0.965  &                    0.911  &                    0.890  &                    0.964  &                    0.823 & 0.911  
\\
Neural Volumes~\cite{neuralvolumes}&                    0.916  &                    0.873  &                    0.910  &                    0.944  &                    0.880  &                    0.888  &                    0.946  &                    0.784  & 0.893
\\
Plenoxels~\cite{fridovich2022plenoxels} &                    0.977  &                    0.933  &                    0.976  &                    0.980  &                    0.976  &                    0.949  &                    0.985  &                    \cellcolor{yellow}0.890  & 0.958
\\
NeRF~\cite{mildenhall2020nerf} &                    0.975  &                    0.925  &                    0.967  &                    0.979  &                    0.968  &                    \cellcolor{red}0.953  &                    0.987  &                    0.869  & 0.953
\\
DVGO~\cite{sun2022direct} &                    0.977  &                    0.930  &                    0.978  &                    0.980  &                    0.976  &                    0.951  &                    0.983  &                    0.879  & 0.957
\\
MipNeRF~\cite{barron2021mip} &                    \cellcolor{yellow}0.981  &                    0.932  &                    0.980  &                    \cellcolor{orange}0.982  &                    0.978  &                    0.959  &                    \cellcolor{orange}0.991  &                    0.882  & 0.961
\\
TensoRF~\cite{chen2022tensorf} &                    \cellcolor{red}0.985  &                    \cellcolor{orange}0.937  &                    \cellcolor{orange}0.982  &                    \cellcolor{orange}0.982  &                    \cellcolor{red}0.983  &                    \cellcolor{yellow}0.952  &                    0.988  &                    \cellcolor{orange}0.895  & \cellcolor{red}0.963
\\
Instant-ngp~\cite{muller2022instant} &                    0.979  &                    \cellcolor{orange}0.937  &                    \cellcolor{yellow}0.981  &                    \cellcolor{orange}0.982  &                    \cellcolor{orange}0.982  &                    0.951  &                    \cellcolor{yellow}0.990  &                    \cellcolor{red}0.896  & \cellcolor{red}0.963
\\
\hline
Tri-MipRF (Ours) &                    \cellcolor{red}0.985  &                    \cellcolor{red}0.939  &                    \cellcolor{red}0.983  &                    \cellcolor{red}0.984  &                    \cellcolor{orange}0.982  &                    \cellcolor{red}0.953  &                    \cellcolor{red}0.992  &                    0.879  & \cellcolor{red}0.963
\\

\multicolumn{9}{c}{} \\
 & \multicolumn{9}{c}{\textbf{LPIPS}} \\
 & \scenename{chair}  & \scenename{drums}  & \scenename{ficus}  & \scenename{hotdog}  & \scenename{lego}  & \scenename{materials}  & \scenename{mic}  & \scenename{ship} & \scenename{Average} 
\\ 
\hline 
SRN~\cite{srn}&                    0.106  &                    0.267  &                    0.149  &                    0.100  &                    0.200  &                    0.174  &                    0.063  &                    0.299  & 0.170
\\
LLFF~\cite{mildenhall2019local}&                    0.064  &                    0.126  &                    0.130  &                    0.061  &                    0.110  &                    0.117  &                    0.084  &                    0.218 & 0.114
\\
Neural Volumes~\cite{neuralvolumes}&                    0.109  &                    0.214  &                    0.162  &                    0.109  &                    0.175  &                    0.130  &                    0.107  &                    0.276  & 0.160
\\
Plenoxels~\cite{fridovich2022plenoxels} &                    0.031  &                    \cellcolor{yellow}0.067  &                    0.026  &                    0.037  &                    0.028  &                    0.057  &                    0.015  &                    0.134  & 0.049
\\
NeRF~\cite{mildenhall2020nerf} &                    0.026  &                    0.071  &                    0.032  &                    0.030  &                    0.031  &                    \cellcolor{orange}0.047  &                    \cellcolor{yellow}0.012  &                    0.150  & 0.050
\\
DVGO~\cite{sun2022direct} &                    0.027  &                    0.077  &                    0.024  &                    0.034  &                    0.028  &                    0.058  &                    0.017  &                    0.161  & 0.053
\\
MipNeRF~\cite{barron2021mip} &                    \cellcolor{orange}0.021  &                    \cellcolor{red}0.065  &                    \cellcolor{red}0.020  &                    \cellcolor{orange}0.027  &                    0.021  &                    \cellcolor{red}0.040  &                    0.009  &                    \cellcolor{yellow}0.138  & \cellcolor{orange}0.043
\\
TensoRF~\cite{chen2022tensorf} &                    \cellcolor{yellow}0.022  &                    0.073  &                    \cellcolor{yellow}0.022  &                    0.032  &                    \cellcolor{yellow}0.018  &                    0.058  &                    0.015  &                    \cellcolor{yellow}0.138  & 0.047
\\
Instant-ngp~\cite{muller2022instant} &                    \cellcolor{yellow}0.022  &                    0.071  &                    0.023  &                    \cellcolor{orange}0.027  &                    \cellcolor{orange}0.017  &                    0.060  &                    \cellcolor{orange}0.010  &                    \cellcolor{red}0.132 & \cellcolor{yellow}0.045 
\\
\hline
Tri-MipRF (Ours) &                    \cellcolor{red}0.016  &                    \cellcolor{orange}0.066  &                    \cellcolor{red}0.020  &                    \cellcolor{red}0.021  &                    \cellcolor{red}0.016  &                    \cellcolor{yellow}0.052  &                    \cellcolor{red}0.008  &                    \cellcolor{orange}0.136  & \cellcolor{red}0.042
\\
\multicolumn{9}{c}{}
