# Supplementary material for: LOD-GS: Level-of-Detail-Sensitive 3D Gaussian Splatting for Detail Conserved Anti-Aliasing
Source: arXiv:2507.00554 source file (2025-08-30)
Supplement: Supplementary file 2 [file multiscale_supp.tex]

& \multicolumn{9}{c}{\textbf{PSNR}} \\
 & \scenename{chair}  & \scenename{drums}  & \scenename{ficus}  & \scenename{hotdog}  & \scenename{lego}  & \scenename{materials}  & \scenename{mic}  & \scenename{ship} & \scenename{Average} 
 \\ 
 \hline 
NeRF w/o $\mathcal{L}_\text{area}$&                    29.92  &                    23.27  &                    27.15  &                    32.00  &                    27.75  &                    26.30  &                    28.40  &                    26.46  & 27.66
\\
NeRF~\cite{mildenhall2020nerf} &                    33.39  &                    25.87  &                    30.37  &                    35.64  &                    31.65  &                    \cellcolor{yellow}30.18  &                    32.60  &                    30.09  & 31.23
\\
MipNeRF~\cite{barron2021mip} &                    \cellcolor{orange}37.14  &                    \cellcolor{orange}27.02  &                    \cellcolor{orange}33.19  &                    \cellcolor{orange}39.31  &                    \cellcolor{orange}35.74  &                    \cellcolor{red}32.56  &                    \cellcolor{orange}38.04  &                    \cellcolor{orange}33.08  & \cellcolor{orange}34.51
\\
\hline
Plenoxels~\cite{fridovich2022plenoxels} &                    32.79  &                    25.25  &                    30.28  &                    34.65  &                    31.26  &                    28.33  &                    31.53  &                    28.59 & 30.34 
\\
TensoRF~\cite{chen2022tensorf} &                    32.47  &                    25.37  &                    31.16  &                    34.96  &                    31.73  &                    28.53  &                    31.48  &                    29.08  & 30.60
\\
Instant-ngp~\cite{muller2022instant} &                    32.95  &                    26.43  &                    30.41  &                    35.87  &                    31.83  &                    29.31  &                    32.58  &                    30.23  & 31.20
\\
Instant-ngp $\uparrow^{5\times}$ &                    \cellcolor{yellow}34.15  &                    26.79  &                    \cellcolor{yellow}31.50  &                    \cellcolor{yellow}36.47  &                    \cellcolor{yellow}32.51  &                    29.49  &                    \cellcolor{yellow}33.81  &                    \cellcolor{yellow}30.78 & \cellcolor{yellow}31.94  
\\
\hline
Tri-MipRF w/o $\mipmap$ &                    33.09  &                    \cellcolor{yellow}26.85  &                    31.07  &                    36.08  &                    32.09  &                    29.85  &                    32.66  &                    30.17  & 31.48
\\
Tri-MipRF (Ours) &                    \cellcolor{red}37.72  &                    \cellcolor{red}28.55  &                    \cellcolor{red}33.77  &                    \cellcolor{red}39.96  &                    \cellcolor{red}36.51  &                    \cellcolor{orange}32.35  &                    \cellcolor{red}38.06  &                    \cellcolor{red}33.59 & \cellcolor{red}35.06  
\\

\multicolumn{9}{c}{} \\
 & \multicolumn{9}{c}{\textbf{SSIM}} \\
 & \scenename{chair}  & \scenename{drums}  & \scenename{ficus}  & \scenename{hotdog}  & \scenename{lego}  & \scenename{materials}  & \scenename{mic}  & \scenename{ship} & \scenename{Average} 
\\ 
\hline 
NeRF w/o $\mathcal{L}_\text{area}$&                    0.944  &                    0.891  &                    0.942  &                    0.959  &                    0.926  &                    0.934  &                    0.958  &                    0.861  &0.927
\\
NeRF~\cite{mildenhall2020nerf} &                    0.971  &                    0.932  &                    0.971  &                    0.979  &                    0.965  &                    \cellcolor{yellow}0.967  &                    0.980  &                    0.900 &0.958  
\\
MipNeRF~\cite{barron2021mip} &                    \cellcolor{orange}0.988  &                    \cellcolor{orange}0.945  &                    \cellcolor{orange}0.984  &                    \cellcolor{orange}0.988  &                    \cellcolor{orange}0.984  &                    \cellcolor{red}0.977  &                    \cellcolor{red}0.993  &                    \cellcolor{orange}0.922  & \cellcolor{orange}0.973
\\
\hline
Plenoxels~\cite{fridovich2022plenoxels} &                    0.968  &                    0.929  &                    0.972  &                    0.976  &                    0.964  &                    0.959  &                    0.979  &                    0.892 & 0.955  
\\
TensoRF~\cite{chen2022tensorf} &                    0.967  &                    0.930  &                    0.974  &                    0.977  &                    0.967  &                    0.957  &                    0.978  &                    0.895  & 0.956 
\\
Instant-ngp~\cite{muller2022instant} &                    0.971  &                    0.940  &                    0.973  &                    0.979  &                    0.966  &                    0.959  &                    0.981  &                    0.904  & 0.959
\\
Instant-ngp $\uparrow^{5\times}$ &                    \cellcolor{yellow}0.979  &                    \cellcolor{yellow}0.943  &                    \cellcolor{yellow}0.978  &                    \cellcolor{yellow}0.982  &                    \cellcolor{yellow}0.972  &                    0.959  &                    \cellcolor{yellow}0.985  &                    \cellcolor{yellow}0.909  & \cellcolor{yellow}0.963
\\
\hline
Tri-MipRF w/o $\mipmap$ &                    0.971  &                    0.941  &                    0.974  &                    0.980  &                    0.967  &                    0.960  &                    0.980  &                    0.901  & 0.959 
\\
Tri-MipRF (Ours) &                    \cellcolor{red}0.990  &                    \cellcolor{red}0.957  &                    \cellcolor{red}0.986  &                    \cellcolor{red}0.989  &                    \cellcolor{red}0.986  &                    \cellcolor{orange}0.972  &                    \cellcolor{orange}0.992  &                    \cellcolor{red}0.935 & \cellcolor{red}0.976  
\\
\multicolumn{9}{c}{} \\
 & \multicolumn{9}{c}{\textbf{LPIPS}} \\
 & \scenename{chair}  & \scenename{drums}  & \scenename{ficus}  & \scenename{hotdog}  & \scenename{lego}  & \scenename{materials}  & \scenename{mic}  & \scenename{ship} & \scenename{Average} 
\\ 
\hline 
NeRF w/o $\mathcal{L}_\text{area}$&                    0.035  &                    0.069  &                    0.032  &                    0.028  &                    0.041  &                    0.045  &                    0.031  &                    0.095  & 0.052
\\
NeRF~\cite{mildenhall2020nerf} &                    0.028  &                    \cellcolor{yellow}0.059  &                    0.026  &                    \cellcolor{yellow}0.024  &                    0.035  &                    \cellcolor{yellow}0.033  &                    0.025  &                    \cellcolor{yellow}0.085  & 0.044
\\
MipNeRF~\cite{barron2021mip} &                    \cellcolor{orange}0.011  &                    \cellcolor{orange}0.044  &                    \cellcolor{red}0.014  &                    \cellcolor{red}0.012  &                    \cellcolor{orange}0.013  &                    \cellcolor{red}0.019  &                    \cellcolor{red}0.007  &                    \cellcolor{red}0.062  & \cellcolor{orange}0.026
\\
\hline
Plenoxels~\cite{fridovich2022plenoxels} &                    0.040  &                    0.070  &                    0.032  &                    0.037  &                    0.038  &                    0.055  &                    0.036  &                    0.104  & 0.051
\\
TensoRF~\cite{chen2022tensorf} &                    0.042  &                    0.075  &                    0.032  &                    0.035  &                    0.036  &                    0.063  &                    0.040  &                    0.112  & 0.054
\\
Instant-ngp~\cite{muller2022instant} &                    0.035  &                    0.066  &                    0.029  &                    0.028  &                    0.040  &                    0.051  &                    0.032  &                    0.095  & 0.047
\\
Instant-ngp $\uparrow^{5\times}$ &                    \cellcolor{yellow}0.025  &                    \cellcolor{yellow}0.059  &                    \cellcolor{yellow}0.023  &                    0.025  &                    \cellcolor{yellow}0.031  &                    0.049  &                    \cellcolor{yellow}0.023  &                    0.089 & \cellcolor{yellow}0.041 
\\
\hline
Tri-MipRF w/o $\mipmap$ &                    0.036  &                    0.066  &                    0.030  &                    0.028  &                    0.039  &                    0.051  &                    0.032  &                    0.099   & 0.048
\\
Tri-MipRF (Ours) &                    \cellcolor{red}0.010  &                    \cellcolor{red}0.042  &                    \cellcolor{red}0.014  &                    \cellcolor{red}0.012  &                    \cellcolor{red}0.012  &                    \cellcolor{orange}0.029  &                    \cellcolor{orange}0.008  &                    \cellcolor{red}0.062  &  \cellcolor{red}0.024 
\\
\multicolumn{9}{c}{}
